# Supplementary material for: PromptRR: Diffusion Models as Prompt Generators for Single Image Reflection Removal
Source: arXiv:2402.02374 source file (2025-08-24)
Supplement: Supplementary file 1 [file 6_supp.tex]

\section{Appendix / supplemental material}

% Optionally include supplemental material (complete proofs, additional experiments and plots) in appendix.
% All such materials \textbf{SHOULD be included in the main submission.}
% In this part, we first introduce the datasets and metrics in subsection~\ref{sec_0}. Then, we 
% provide more details of MSA and FFN in subsection~\ref{sec_1} and illustrate more details of diffusion models we use in our method in subsection~\ref{sec_2}. Finally, we show more visual comparisons in subsection~\ref{sec_3}.

In this part, we first provide more details of MSA and FFN in subsection~\ref{sec_1}. Then, we discuss more details of diffusion models we use in our method in subsection~\ref{sec_2}. Finally, we show more visual comparisons in subsection~\ref{sec_3}.

% \subsection{Datasets and Metrics}\label{sec_0}

% We conduct experiments on popular benchmarks. Following previous works~\cite{hu2021trash,song2023robust}, we train our networks on a dataset consisting of a combination of synthetic and real-world data. For the synthetic training data, we adopt the PASCAL VOC dataset~\cite{Everingham2010} to synthesize $7,643$ images using the data-generation method described in \cite{fan2017generic}. For the real-world data, we adopt $90$ real-world training images from~\cite{zhang2018single}. In the testing phase, we evaluate models on three commonly used real-world datasets, Nature~\cite{Li_2020_CVPR}, $SIR^{2}$~\cite{Wan_2017_iccv}, and Real dataset~\cite{zhang2018single}. The $SIR^{2}$ dataset comprises three subsets, namely \textit{PostCard}, \textit{SolidObject}, and \textit{WildScene}. In addition, PSNR~\cite{huynh2008scope} and SSIM~\cite{wang2004image} are used as the metrics for performance evaluation.

\subsection{More Details of MSA and FFN in Transformer}\label{sec_1}

\begin{figure}[ht]
\begin{center}
   \includegraphics[width=0.6\textwidth]{images_supp/supp_msa_ffn_v5.pdf}
	  % \vspace{-0.1in}
   % \vspace{-3mm}
	\caption{The structure of the proposed prompt multi-head self-attention and prompt feed-forward network. The black dotted boxes indicate our prompt interaction and injection module. Removing the black dashed boxes in Fig~(a) and (b), the corresponding modules degenerate to the MDTA and GDFN respectively.}
	\label{fig:units_promptformer}
 \end{center}
   % \vspace{-5mm}
\end{figure}
\quad Our proposed transformer-based prompt block consists of prompt multi-head self-attention and prompt feed-forward network, which are built based on existing multi-dconv head transposed attention (MDTA) and gated-dconv feed-forward network (GDFN)~\cite{zamir2022restormer}, respectively. In this section, we provide more details of MDTA and GDFN. As shown in Fig.~\ref{fig:units_promptformer} (a), MDTA mainly performs self-attention across features' channels rather than the spatial dimension to reduce the time
and memory complexity. Specifically, given the input feature $\mathbf{X} \in \mathbb{R}^{ C \times H \times W}$, it is first passed into a normalization layer to obtain the normalized feature $\mathbf{X}^{\prime} \in \mathbb{R}^{C \times H \times W }$. Then, a $1\times1$ convolution followed by a $3\times3$ depth-wise convolution is used to generate Query ($\mathbf{Q}$), Key ($\mathbf{K}$), and Value ($\mathbf{V}$), \ie $\mathbf{Q}=W_{3\times3}^{q}W_{1\times1}^{q}\mathbf{X}^{\prime}$, $\mathbf{K}=W_{3\times3}^{k}W_{1\times1}^{k}\mathbf{X}^{\prime}$, $\mathbf{V}=W_{3\times3}^{v}W_{1\times1}^{v}\mathbf{X}^{\prime}$, where $W_{1\times1}(.)$ and $W_{3\times3}(.)$ denote $1\times1$ convolution and $3\times3$ depth-wise convolution, respectively. After that, the reshaped $\hat{\mathbf{Q}}$ and $\hat{\mathbf{K}}$ are used to calculate channel-wise attention matrix $\mathbf{M}\in \mathbb{R}^{C \times C}$. The process of MDTA can be formulated as:
\begin{equation}
\begin{aligned}
&\operatorname{Att}(\hat{\mathbf{Q}}, \hat{\mathbf{K}}, \hat{\mathbf{V}})=\operatorname{Softmax}\left(\frac{\hat{\mathbf{Q}}\hat{\mathbf{K}}^{\top}}{\alpha}\right) \hat{\mathbf{V}}, \\
& \hat{\mathbf{X}} = W_{1\times1}\operatorname{Att}(\hat{\mathbf{Q}},\hat{\mathbf{K}},\hat{\mathbf{V}}) + \mathbf{X},
\end{aligned}
\end{equation}
where $\hat{\mathbf{Q}} \in \mathbb{R}^{C \times(HW)} $, $\hat{\mathbf{K}} \in \mathbb{R}^{C\times(HW)}$, and $\hat{\mathbf{V}} \in \mathbb{R}^{C\times(HW)}$ refer to reshaped tensors of $\mathbf{Q}$, $\mathbf{K}$, and $\mathbf{V}$, respectively. $\mathbf{X}$ and  $\hat{\mathbf{X}}$ are input and output features. 
As shown in Fig.~\ref{fig:units_promptformer} (b), GDFN mainly adopts a gating mechanism to control the useful information in the network. Given $\mathbf{X} \in \mathbb{R}^{ C \times H \times W }$ as input, the 
process of GDFN is formulated as:
\begin{equation}
\begin{aligned}
&\text{Gate}(\mathbf{X}) =\phi\left(W_{3\times3}^{1} W_{1\times1}^{1}(LN(\mathbf{X}))\right) \odot (W_{3\times3}^{2} W_{1\times1}^{2}(LN(\mathbf{X}))), \\
&\hat{\mathbf{X}} = W_{1\times1}\text {Gate}(\mathbf{X})+\mathbf{X},
\end{aligned}
\end{equation}
where $\hat{\mathbf{X}} \in \mathbb{R}^{C\times H \times W }$ represents the output features, $\text{Gate}(\cdot)$ refers to the  gated mechanism. $W_{1\times1}(\cdot)$ and $W_{3\times3}(\cdot)$ denote $1\times1$ convolution and $3\times3$ depth-wise convolution. LN is the layer normalization, $\odot$ is the element-wise multiplication operation, and $\phi(\cdot)$ is the GELU activation function.

\begin{algorithm*}[t]
\hspace*{\algorithmicindent}\noindent \textbf{Input:} reflection image $I$, ground-truth image $I_{gt}$, pre-trained frequency prompt encoder $\operatorname{FPE_{pre}}$, and conditional frequency prompt encoder $\operatorname{FPE_{con}}$.
\caption{Diffusion training (diffusion process)}\label{algo_train}
\begin{algorithmic}[1]
        \While{not converged}
        \State $\mathbf{P}^{l}_0,\mathbf{P}^{h}_0 = \operatorname{FPE_{pre}}(\operatorname{Concat}(I_{gt},I)). $
        \State $\mathbf{P}^{l}_c,\mathbf{P}^{h}_c = \operatorname{FPE_{con}}(I). $
        \State $t \sim \text{Uniform}\{1, \ldots, T\}$
        \State $\bm{\epsilon^{l}} \sim \mathcal{N}(\mathbf{0},\mathbf{I})$
        \State $\bm{\epsilon^{h}} \sim \mathcal{N}(\mathbf{0},\mathbf{I})$
        \State $\mathbf{P}^{l}_{t+1} = \sqrt{\bar{\alpha}^{l}_t} \mathbf{P}^{l}_0+\sqrt{1-\bar{\alpha}^{l}_t} \bm{\epsilon^{l}}$
        \State $\mathbf{P}^{h}_{t+1} = \sqrt{\bar{\alpha}^{h}_t} \mathbf{P}^{h}_0+\sqrt{1-\bar{\alpha}^{h}_t} \bm{\epsilon^{h}}$
        \State $\mathbf{e}^{l}_t = \bm{\epsilon^{l}}_\theta\left(\mathbf{P}^{l}_c, \mathbf{P}^{l}_{t+1}, t\right)$
        \State $\mathbf{e}^{h}_t = \bm{\epsilon^{h}}_\theta\left(\mathbf{P}^{h}_c, \mathbf{P}^{h}_{t+1}, t\right)$  
      \State Perform gradient descent steps on $\nabla_\theta 
        \;\mathcal{L}_{\mathrm{diff}}(\theta)$ 
     % \EndIf
        \EndWhile
      \\ \textbf{Output:} the trained low-frequency prompt generation diffusion model $\bm{\epsilon^{l}}_\theta$, the trained high-frequency prompt generation diffusion model $\bm{\epsilon^{h}}_\theta$,  the trained conditional frequency prompt encoder $\operatorname{FPE_{con}}$.    
      % \\ $\textbf{return}\;\; \theta$ 
\end{algorithmic}
  % \vspace{-2mm}
\end{algorithm*}

\begin{algorithm*}[t]
\hspace*{\algorithmicindent}\noindent \textbf{Input:} reflection image $I$, the number of implicit sampling steps $T$, the trained low-frequency prompt generation diffusion model $\bm{\epsilon^{l}}_\theta$, the trained high-frequency prompt generation diffusion model $\bm{\epsilon^{h}}_\theta$, and the trained conditional frequency prompt encoder $\operatorname{FPE_{con}}$.
\caption{Diffusive sampling (generation process)}\label{algo}
\begin{algorithmic}[1]
        \State $\mathbf{P}^{l}_c,\mathbf{P}^{h}_c = \operatorname{FPE_{con}}(I). $
      \State $\mathbf{P}^{l}_T \sim \mathcal{N}(\mathbf{0}, \mathbf{I})$
     \State $\mathbf{P}^{h}_T \sim \mathcal{N}(\mathbf{0}, \mathbf{I})$
      \For{$t =T, \ldots, 1$}
        \State $\mathbf{e}^{l}_{t-1} = \bm{\epsilon^{l}}_\theta\left(\mathbf{P}^{l}_c, \mathbf{P}^{l}_t,  t \right)$
        \State $\mathbf{P}^{l}_{t-1} \!\!= \!\!\sqrt{\bar{\alpha}^{l}_{t-{1}}}\left(\frac{\mathbf{P}^{l}_{t}-\sqrt{1-\bar{\alpha}^{l}_t} \cdot \mathbf{e}^{l}_{t-1}}{\sqrt{\bar{\alpha}^{l}_t}}\right)
       \! +\!\sqrt{1-\bar{\alpha}^{l}_{t-{1}}} \cdot \mathbf{e}^{l}_{t-1}$

        \State $\mathbf{e}^{h}_{t-1} = \bm{\epsilon^{h}}_\theta\left(\mathbf{P}^{h}_c, \mathbf{P}^{h}_t,  t \right)$
        \State $\mathbf{P}^{h}_{t-1} \!\!= \!\!\sqrt{\bar{\alpha}^{h}_{t-{1}}}\left(\frac{\mathbf{P}^{h}_{t}-\sqrt{1-\bar{\alpha}^{h}_t} \cdot \mathbf{e}^{h}_{t-1}}{\sqrt{\bar{\alpha}^{h}_t}}\right)
       \! +\!\sqrt{1-\bar{\alpha}^{h}_{t-{1}}} \cdot \mathbf{e}^{h}_{t-1}$
      \EndFor
      % \State \Return $\mathbf{P}^{l}_0$, $\mathbf{P}^{h}_0$

     \\ \textbf{Output:} low-frequency prompt $\mathbf{P}^{l}_0$, high-frequency prompt $\mathbf{P}^{h}_0$. 
\end{algorithmic}
  % \vspace{-1mm}
\end{algorithm*}

\subsection{More Details of Diffusion Models}\label{sec_2}

\quad In our method, we use two diffusion models (DMs) as prompt generators to generate low-frequency and high-frequency prompts respectively for subsequent prompt-guide restoration. DMs contain the diffusion process and the generation process. These two processes are illustrated in 
Algorithm~\ref{algo_train} and Algorithm~\ref{algo}, respectively.

\subsection{More Visual Results}\label{sec_3}

\quad This section presents additional visual comparisons for reflection removal in different datasets, including \textit{Nature}~\cite{Li_2020_CVPR}, \textit{PostCard}~\cite{Wan_2017_iccv}, \textit{SolidObject}~\cite{Wan_2017_iccv}, and \textit{WildScene}~\cite{Wan_2017_iccv}, and \textit{Real}~\cite{zhang2018single}. Specifically, the comparison methods are WY19~\cite{Wei_2019_CVPR}, WT19~\cite{Wen_2019_CVPR}, LY20~\cite{Li_2020_CVPR}, ZS21~\cite{Zheng_2021_CVPR}, CL21~\cite{Chang2021_wacv}, HG21~\cite{hu2021trash}, Uformer~\cite{wang2022uformer}, Restormer~\cite{zamir2022restormer}, and RSIRR~\cite{song2023robust}.

\textbf{Visual Results on \textit{Nature}:} Figure \ref{results_fig1}. \\

\textbf{Visual Results on \textit{PostCard}:} Figure \ref{results_fig3}. \\

\textbf{Visual Results on \textit{SolidObject}:} Figure \ref{results_fig6}.\\

\textbf{Visual Results on \textit{WildScene}:} Figure \ref{results_fig7}. \\

\textbf{Visual Results on \textit{Real}:} Figure \ref{results_fig10}.\\

% \subsection{Limitations and Future Work}
% Our PromptRR has achieved better performance than previous SIRR methods, but there is still room for improvement. For instance, integrating techniques like contrastive learning~\cite{wu2021contrastive}or new frameworks like Mamba~\cite{gu2023mamba} into PromptRR could enhance its performance further. Additionally, while PromptRR is tailored for image scenery, its capability to handle video reflection removal is still under investigation. Extending PromptRR to address this challenge is an important direction for future research.

% \newpage

\def \rootnaturev2 {images_supp/datasets-v2/Nature/origin_img_with_box/}
\begin{figure*}[ht]
    \centering
    \subfloat[Input (PSNR: 23.55)]{
    \includegraphics[width=0.24\linewidth]{\rootnaturev2 input/input_1-2_71.pdf}
    }\hspace{-5pt}
    \subfloat[WY19 (PSNR: 19.37)]{
        \includegraphics[width=0.24\linewidth]{\rootnaturev2 WY19/WY19_1-2_71.pdf}
    }\hspace{-5pt}
    \subfloat[WT19~(PSNR: 10.05)]{ 
        \includegraphics[width=0.24\linewidth]{\rootnaturev2  WT19/WT19_1-2_71.pdf}
    }\hspace{-5pt}
    \subfloat[LY20~(PSNR: 21.95)]{
        \includegraphics[width=0.24\linewidth]{\rootnaturev2 LY20/LY20_1-2_71.pdf}
    } \\
    % \hspace{-5pt}
    \subfloat[ZS21~(PSNR: 16.79)]{
        \includegraphics[width=0.24\linewidth]{\rootnaturev2 ZS21/ZS21_1-2_71.pdf}
    } \hspace{-5pt}
    \subfloat[CL21~(PSNR: 21.94)]{
        \includegraphics[width=0.24\linewidth]{\rootnaturev2 CL21/CL21_1-2_71.pdf}
    } \hspace{-5pt}
    \subfloat[HG21~(PSNR: 19.24)]{
        \includegraphics[width=0.24\linewidth]{\rootnaturev2 HG21/HG21_1-2_71.pdf}
    }\hspace{-5pt}
    \subfloat[Uformer~(PSNR: 22.43)]{
        \includegraphics[width=0.24\linewidth]{\rootnaturev2 Uformer/Uformer_1-2_71.pdf}
    } \\
    \subfloat[Restormer~(PSNR: 23.50)]{
        \includegraphics[width=0.24\linewidth]{\rootnaturev2 Restormer/Restormer_1-2_71.pdf}
    }\hspace{-5pt}
    \subfloat[RSIRR~(PSNR: 22.69)]{
        \includegraphics[width=0.24\linewidth]{\rootnaturev2 RSIRR/RSIRR_1-2_71.pdf} 
    }\hspace{-5pt}
        \subfloat[Ours (PSNR: 23.57)]{
        \includegraphics[width=0.24\linewidth]{\rootnaturev2 PromptRR/PromptRR_1-2_71.pdf} 
    }\hspace{-5pt}
        \subfloat[GT]{
        \includegraphics[width=0.24\linewidth]{\rootnaturev2 GT/GT_1-2_71.pdf} 
    }   
    \vspace{-2mm}
    \caption{Visual comparison on \textit{Nature}~\cite{Li_2020_CVPR} dataset. \textbf{Zoom-in for better details}.}
    \label{results_fig1}
    \vspace{-2mm}
\end{figure*}

\def \rootpostcardv2 {images_supp/datasets-v2/postcard/origin_img_with_box/}
\begin{figure*}[ht]
    \centering
    \subfloat[Input (PSNR: 21.23)]{
    \includegraphics[width=0.24\linewidth]{\rootpostcardv2 input/input_ea-5-m-11.pdf}
    }\hspace{-5pt}
    \subfloat[WY19 (PSNR: 20.16)]{
        \includegraphics[width=0.24\linewidth]{\rootpostcardv2 WY19/WY19_ea-5-m-11.pdf}
    }\hspace{-5pt}
    \subfloat[WT19 (PSNR: 7.17)]{ 
        \includegraphics[width=0.24\linewidth]{\rootpostcardv2  WT19/WT19_ea-5-m-11.pdf}
    }\hspace{-5pt}
    \subfloat[LY20 (PSNR: 17.42)]{
        \includegraphics[width=0.24\linewidth]{\rootpostcardv2 LY20/LY20_ea-5-m-11.pdf}
    } \\
    % \hspace{-5pt}
    \subfloat[ZS21 (PSNR: 16.10)]{
        \includegraphics[width=0.24\linewidth]{\rootpostcardv2 ZS21/ZS21_ea-5-m-11.pdf}
    } \hspace{-5pt}
    \subfloat[CL21 (PSNR: 19.34)]{
        \includegraphics[width=0.24\linewidth]{\rootpostcardv2 CL21/CL21_ea-5-m-11.pdf}
    } \hspace{-5pt}
    \subfloat[HG21 (PSNR: 21.11)]{
        \includegraphics[width=0.24\linewidth]{\rootpostcardv2 HG21/HG21_ea-5-m-11.pdf}
    }\hspace{-5pt}
    \subfloat[Uformer (PSNR: 16.95)]{
        \includegraphics[width=0.24\linewidth]{\rootpostcardv2 Uformer/Uformer_ea-5-m-11.pdf}
    } \\
    \subfloat[Restormer (PSNR: 11.05)]{
        \includegraphics[width=0.24\linewidth]{\rootpostcardv2 Restormer/Restormer_ea-5-m-11.pdf}
    }\hspace{-5pt}
    \subfloat[RSIRR (PSNR: 19.06)]{
        \includegraphics[width=0.24\linewidth]{\rootpostcardv2 RSIRR/RSIRR_ea-5-m-11.pdf} 
    }\hspace{-5pt}
        \subfloat[Ours (PSNR: 28.19)]{
        \includegraphics[width=0.24\linewidth]{\rootpostcardv2 PromptRR/PromptRR_ea-5-m-11.pdf} 
    }\hspace{-5pt}
        \subfloat[GT]{
        \includegraphics[width=0.24\linewidth]{\rootpostcardv2 GT/GT_ea-5-m-11.pdf} 
    }   
    \vspace{-2mm}
    \caption{Visual comparison on \textit{PostCard}~\cite{Wan_2017_iccv} dataset. \textbf{Zoom-in for better details}.}
    \vspace{-2mm}
    \label{results_fig3}
\end{figure*}

\newpage

\def \rootsolidobjectv2 {images_supp/datasets-v2/solidobject/origin_img_with_box/}

\begin{figure*}[ht]
    \centering
    \subfloat[Input (PSNR: 22.56)]{
    \includegraphics[width=0.24\linewidth]{\rootsolidobjectv2 input/input_14-Focus-11-m.pdf}
    }\hspace{-5pt}
    \subfloat[WY19~(PSNR: 22.23)]{
        \includegraphics[width=0.24\linewidth]{\rootsolidobjectv2 WY19/WY19_14-Focus-11-m.pdf}
    }\hspace{-5pt}
    \subfloat[WT19~(PSNR: 10.10)]{ 
        \includegraphics[width=0.24\linewidth]{\rootsolidobjectv2  WT19/WT19_14-Focus-11-m.pdf}
    }\hspace{-5pt}
    \subfloat[LY20~(PSNR: 23.36)]{
        \includegraphics[width=0.24\linewidth]{\rootsolidobjectv2 LY20/LY20_14-Focus-11-m.pdf}
    } \\
    % \hspace{-5pt}
    \subfloat[ZS21~(PSNR: 18.51)]{
        \includegraphics[width=0.24\linewidth]{\rootsolidobjectv2 ZS21/ZS21_14-Focus-11-m.pdf}
    } \hspace{-5pt}
    \subfloat[CL21~(PSNR: 23.92)]{
        \includegraphics[width=0.24\linewidth]{\rootsolidobjectv2 CL21/CL21_14-Focus-11-m.pdf}
    } \hspace{-5pt}
    \subfloat[HG21~(PSNR: 21.84)]{
        \includegraphics[width=0.24\linewidth]{\rootsolidobjectv2 HG21/HG21_14-Focus-11-m.pdf}
    }\hspace{-5pt}
    \subfloat[Uformer~(PSNR: 22.63)]{
        \includegraphics[width=0.24\linewidth]{\rootsolidobjectv2 Uformer/Uformer_14-Focus-11-m.pdf}
    } \\
    \subfloat[Restormer~(PSNR: 25.23)]{
        \includegraphics[width=0.24\linewidth]{\rootsolidobjectv2 Restormer/Restormer_14-Focus-11-m.pdf}
    }\hspace{-5pt}
    \subfloat[RSIRR~(PSNR: 24.98)]{
        \includegraphics[width=0.24\linewidth]{\rootsolidobjectv2 RSIRR/RSIRR_14-Focus-11-m.pdf} 
    }\hspace{-5pt}
        \subfloat[Ours (PSNR: 25.84)]{
        \includegraphics[width=0.24\linewidth]{\rootsolidobjectv2 PromptRR/PromptRR_14-Focus-11-m.pdf} 
    }\hspace{-5pt}
        \subfloat[GT]{
        \includegraphics[width=0.24\linewidth]{\rootsolidobjectv2 GT/GT_14-Focus-11-m.pdf} 
    }   
    % \vspace{-3mm}
    \caption{Visual comparison on \textit{SolidObject}~\cite{Wan_2017_iccv} dataset. \textbf{Zoom-in for better details}.}
    \vspace{-2mm}
    \label{results_fig6}
\end{figure*}

% \newpage

\def \rootwildv2 {images_supp/datasets-v2/wild_v2/}
\begin{figure*}[ht]
    \centering
    \subfloat[Input (PSNR: 14.80)]{
    \includegraphics[width=0.24\linewidth]{\rootwildv2 input_22s-m.pdf}
    }\hspace{-5pt}
    \subfloat[WY19~(PNSR: 21.31)]{
        \includegraphics[width=0.24\linewidth]{\rootwildv2 WY19_22s-m.pdf}
    }\hspace{-5pt}
    \subfloat[WT19~(PNSR: 12.99)]{ 
        \includegraphics[width=0.24\linewidth]{\rootwildv2  WT19_22s-m.pdf}
    }\hspace{-5pt}
    \subfloat[LY20~(PNSR: 23.78)]{
        \includegraphics[width=0.24\linewidth]{\rootwildv2 LY20_22s-m.pdf}
    } \\
    % \hspace{-5pt}
    \subfloat[ZS21~(PNSR: 22.91)]{
        \includegraphics[width=0.24\linewidth]{\rootwildv2 ZS21_22s-m.pdf}
    } \hspace{-5pt}
    \subfloat[CL21~(PNSR: 19.88)]{
        \includegraphics[width=0.24\linewidth]{\rootwildv2 CL21_22s-m.pdf}
    } \hspace{-5pt}
    \subfloat[HG21~(PNSR: 17.14)]{
        \includegraphics[width=0.24\linewidth]{\rootwildv2 HG21_22s-m.pdf}
    }\hspace{-5pt}
    \subfloat[Uformer~(PNSR: 18.17)]{
        \includegraphics[width=0.24\linewidth]{\rootwildv2 Uformer_22s-m.pdf}
    } \\
    \subfloat[Restormer~(PNSR: 29.55)]{
        \includegraphics[width=0.24\linewidth]{\rootwildv2 Restormer_22s-m.pdf}
    }\hspace{-5pt}
    \subfloat[RSIRR~(PNSR: 16.99)]{
        \includegraphics[width=0.24\linewidth]{\rootwildv2 RSIRR_22s-m.pdf} 
    }\hspace{-5pt}
        \subfloat[Ours (PNSR: 31.07)]{
        \includegraphics[width=0.24\linewidth]{\rootwildv2 PromptRR_22s-m.pdf} 
    }\hspace{-5pt}
        \subfloat[GT]{
        \includegraphics[width=0.24\linewidth]{\rootwildv2 GT_22s-m.pdf} 
    }   
    \vspace{-3mm}
    \caption{Visual comparison on \textit{WildScene}~\cite{Wan_2017_iccv} dataset. \textbf{Zoom-in for better details}.}
    \vspace{-3mm}
    \label{results_fig7}
\end{figure*}

\newpage

\def \rootrealv2 {images_supp/datasets-v2/real/origin_img_with_box/}

\begin{figure*}[ht]
    \centering
    \subfloat[Input (PSNR: 18.06)]{
    \includegraphics[width=0.24\linewidth]{\rootrealv2 input/input_89.pdf}
    }\hspace{-5pt}
    \subfloat[WY19~(PSNR: 19.61)]{
        \includegraphics[width=0.24\linewidth]{\rootrealv2 WY19/WY19_89.pdf}
    }\hspace{-5pt}
    \subfloat[WT19~(PSNR: 7.60)]{ 
        \includegraphics[width=0.24\linewidth]{\rootrealv2  WT19/WT19_89.pdf}
    }\hspace{-5pt}
    \subfloat[LY20~(PSNR: 20.36)]{
        \includegraphics[width=0.24\linewidth]{\rootrealv2 LY20/LY20_89.pdf}
    } \\
    % \hspace{-5pt}
    \subfloat[ZS21~(PSNR: 17.72)]{
        \includegraphics[width=0.24\linewidth]{\rootrealv2 ZS21/ZS21_89.pdf}
    } \hspace{-5pt}
    \subfloat[CL21~(PSNR: 20.87)]{
        \includegraphics[width=0.24\linewidth]{\rootrealv2 CL21/CL21_89.pdf}
    } \hspace{-5pt}
    \subfloat[HG21~(PSNR: 22.45)]{
        \includegraphics[width=0.24\linewidth]{\rootrealv2 HG21/HG21_89.pdf}
    }\hspace{-5pt}
    \subfloat[Uformer~(PSNR: 18.37)]{
        \includegraphics[width=0.24\linewidth]{\rootrealv2 Uformer/Uformer_89.pdf}
    } \\
    \subfloat[Restormer~(PSNR: 18.67)]{
        \includegraphics[width=0.24\linewidth]{\rootrealv2 Restormer/Restormer_89.pdf}
    }\hspace{-5pt}
    \subfloat[RSIRR~(PSNR: 24.77)]{
        \includegraphics[width=0.24\linewidth]{\rootrealv2 RSIRR/RSIRR_89.pdf} 
    }\hspace{-5pt}
        \subfloat[Ours (PSNR: 26.15)]{
        \includegraphics[width=0.24\linewidth]{\rootrealv2 PromptRR/PromptRR_89.pdf} 
    }\hspace{-5pt}
        \subfloat[GT]{
        \includegraphics[width=0.24\linewidth]{\rootrealv2 GT/GT_89.pdf} 
    }   
    % \vspace{-2mm}
    \caption{Visual comparison on \textit{Real}~\cite{zhang2018single} dataset. \textbf{Zoom-in for better details}.}
    % \vspace{-2mm}
    \label{results_fig10}
\end{figure*}
